# Supplementary material for: A Hierarchy of Non-Equilibrium Two-Phase Flow Models
Source: arXiv:1804.05241 source file (2018-04-14)
Supplement: Supplementary file 1 [file supplement_partials.pdf]

**Supplementary Material for**
**"A Hierarchy of Non-Equilibrium Two-Phase Flow Models"**

Gaute Linga April 13, 2018

## Thermodynamic differentials

We here present, for a single-phase, single-component equation of state, the thermodynamic differentials involving the following *primary thermodynamic variables*:

$e$ — internal energy per mass,

$s$ — entropy per mass,

$p$ — pressure,

$\rho$ — density, and

$T$ — temperature.

Differentials of other variables, like chemical potential $\mu$ and enthalpy per mass $h$, can be found using linear combination of the forthcoming expressions. The variables are expressed using a minimal set of *thermodynamic derivatives*:

$c$ — thermodynamic speed of sound, defined in (19);

$\Gamma$ — first Grüneisen coefficient, defined in (10);

$C_p$ — specific isobaric heat capacity, defined in (22).

In the following we summarize the consistent set of termodynamic differentials of all triads from the list of primitive variables above.

- $(e, s, p)$:

$$\left(\frac{\partial e}{\partial p}\right)_s = \frac{p}{\rho^2 c^2} \tag{1}$$

$$\left(\frac{\partial e}{\partial s}\right)_p = T\left[1 - \frac{\Gamma p}{\rho c^2}\right] \tag{2}$$

$$\left(\frac{\partial p}{\partial s}\right)_e = T\rho\left[\Gamma - \frac{\rho c^2}{p}\right] \tag{3}$$

- $(e, s, \rho)$:

$$\left(\frac{\partial e}{\partial s}\right)_\rho = T \tag{4}$$

$$\left(\frac{\partial e}{\partial \rho}\right)_s = \frac{p}{\rho^2} \tag{5}$$

$$\left(\frac{\partial \rho}{\partial s}\right)_e = -\frac{T\rho^2}{p} \tag{6}$$

- $(e, s, T)$:

$$\left(\frac{\partial e}{\partial T}\right)_s = \frac{p}{\Gamma\rho T} \tag{7}$$

$$\left(\frac{\partial e}{\partial s}\right)_T = T - \frac{p}{\Gamma\rho C_p} - \frac{\Gamma p T}{\rho c^2} \tag{8}$$

$$\left(\frac{\partial T}{\partial s}\right)_e = \frac{\Gamma\rho T}{p}\left[\frac{p}{\Gamma\rho C_p} + \frac{\Gamma p T}{\rho c^2} - T\right] \tag{9}$$

- $(e, p, \rho)$:

$$\left(\frac{\partial p}{\partial e}\right)_\rho = \Gamma\rho \tag{10}$$

$$\left(\frac{\partial p}{\partial \rho}\right)_e = c^2 - \frac{\Gamma p}{\rho} \tag{11}$$

$$\left(\frac{\partial e}{\partial \rho}\right)_p = \frac{1}{\rho}\left[\frac{p}{\rho} - \frac{c^2}{\Gamma}\right] \tag{12}$$

- $(e, p, T)$:

$$\left(\frac{\partial e}{\partial p}\right)_T = \frac{1}{\rho c^2}\left[-\Gamma C_p T + \frac{p}{\rho} + \frac{\Gamma^2 C_p p T}{\rho c^2}\right] \tag{13}$$

$$\left(\frac{\partial e}{\partial T}\right)_p = C_p\left[1 - \frac{\Gamma p}{\rho c^2}\right] \tag{14}$$

$$\left(\frac{\partial p}{\partial T}\right)_e = \frac{\Gamma p - \rho c^2}{-\Gamma T + \frac{p}{\rho C_p} + \frac{\Gamma^2 p T}{\rho c^2}} \tag{15}$$

- $(e, \rho, T)$:

$$\left(\frac{\partial e}{\partial T}\right)_\rho = \left[\frac{1}{C_p} + \frac{\Gamma^2 T}{c^2}\right]^{-1} \tag{16}$$

$$\left(\frac{\partial e}{\partial \rho}\right)_T = \frac{1}{\rho}\left(\frac{p}{\rho} - \left[\frac{1}{\Gamma C_p T} + \frac{\Gamma}{c^2}\right]^{-1}\right) \tag{17}$$

$$\left(\frac{\partial T}{\partial \rho}\right)_e = \frac{1}{\rho}\left[\Gamma T - \frac{p}{\rho C_p} - \frac{\Gamma^2 p T}{\rho c^2}\right] \tag{18}$$

- $(s, p, \rho)$:

$$\left(\frac{\partial p}{\partial \rho}\right)_s = c^2 \tag{19}$$

$$\left(\frac{\partial p}{\partial s}\right)_\rho = \Gamma \rho T \tag{20}$$

$$\left(\frac{\partial \rho}{\partial s}\right)_p = -\frac{\Gamma \rho T}{c^2} \tag{21}$$

- $(s, p, T)$:

$$\left(\frac{\partial s}{\partial T}\right)_p = \frac{C_p}{T} \tag{22}$$

$$\left(\frac{\partial s}{\partial p}\right)_T = -\frac{\Gamma C_p}{\rho c^2} \tag{23}$$

$$\left(\frac{\partial T}{\partial p}\right)_s = \frac{\Gamma T}{\rho c^2} \tag{24}$$

- $(s, \rho, T)$:

$$\left(\frac{\partial T}{\partial \rho}\right)_s = \frac{\Gamma T}{\rho} \tag{25}$$

$$\left(\frac{\partial T}{\partial s}\right)_\rho = \frac{T}{C_p} + \frac{\Gamma^2 T^2}{c^2} \tag{26}$$

$$\left(\frac{\partial s}{\partial \rho}\right)_T = -\frac{1}{\rho}\left[\frac{1}{\Gamma C_p} + \frac{\Gamma T}{c^2}\right]^{-1} \tag{27}$$

- $(p, \rho, T)$:

$$\left(\frac{\partial \rho}{\partial T}\right)_p = -\frac{\Gamma \rho C_p}{c^2} \tag{28}$$

$$\left(\frac{\partial \rho}{\partial p}\right)_T = \frac{1}{c^2}\left[1 + \frac{\Gamma^2 C_p T}{c^2}\right] \tag{29}$$

$$\left(\frac{\partial p}{\partial T}\right)_\rho = \rho\left[\frac{1}{\Gamma C_p} + \frac{\Gamma T}{c^2}\right]^{-1} \tag{30}$$
